# Supplementary material for: Quasi-1D Coulomb drag between spin-polarized quantum wires
Source: arXiv:2506.14967 ancillary file (2025-06-17)
Supplement: Supplementary file 1 [file SM_Spin_polarization_drag.pdf]

# Supplementary Materials: “Quasi 1D Coulomb drag between spin-polarized quantum wires”

Mingyang Zheng,<sup>1</sup> Rebika Makaju,<sup>1</sup> Rasul Gazizulin,<sup>1,2</sup> Alex Levchenko,<sup>3</sup> Sadvikas J. Addamane,<sup>4</sup> and Dominique Laroche<sup>1,\*</sup>

<sup>1</sup>*Department of Physics, University of Florida, Gainesville, FL 32611, USA*

<sup>2</sup>*National High Magnetic Field Laboratory High B/T Facility,  
University of Florida, Gainesville, FL 32611, USA*

<sup>3</sup>*Department of Physics, University of Wisconsin–Madison, Madison, WI 53706, USA*

<sup>4</sup>*Center for Integrated Nanotechnologies, Sandia National Laboratories, Albuquerque, NM 87185, USA*

## DEVICE FABRICATION

The vertically-integrated double quantum wires used in this Letter are patterned on an n-doped GaAs/AlGaAs electron bilayer heterostructure (wafer VA1110). The two 18 nm wide quantum wells are separated by a 15 nm wide Al<sub>0.3</sub>Ga<sub>0.7</sub>As barrier. The unpatterned density and mobility of the GaAs quantum well are  $2.98 \times 10^{11} \text{ cm}^{-2}$ ,  $\mu = 7.4 \times 10^4 \text{ cm}^2/\text{V} \cdot \text{s}$ , respectively. Two sets of two split gates are deposited using electron beam lithography on the upper and the lower side of the sample using an epoxy-bound-and-stop-etch (EBASE) process. These gates define two wires that are  $\sim 5 \mu\text{m}$  long and  $\sim 0.6 \mu\text{m}$  wide. More details on the fabrication process are presented elsewhere [1]. A microscopy image of the finished vertically-integrated quantum wires is presented in Fig. S1(a), along with a zoom-in microscopy image of the wire overlapping region in Fig. S1(b). In Fig. S1(b), the lower wire design is overlapped with the zoom-in microscopy image, demonstrating the good alignment between the two quantum wires.

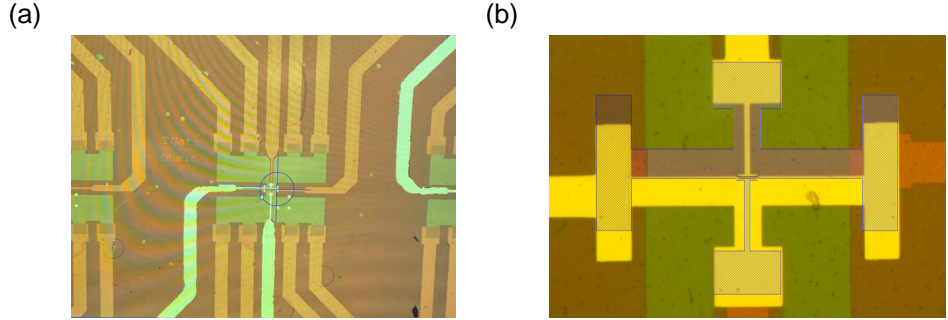

Fig. S1. Optical microscopy image and design of the vertical device. (a) Optical microscopy image of the vertical device. (b) Zoom-in image of the wire region. The wires overlapping region is shown. The lower wire design is overlapped with the zoom-in microscopy image.

## ADDITIONAL DEVICE CHARACTERIZATION

A circuit diagram of the Coulomb drag measurement scheme utilizing a virtual ground on the drag side is presented in Fig. S2, where the drive current is applied on the top wire and the drag voltage is measured on the bottom wire. This setup ensures that no accidental bias is applied to the drag wire throughout the measurement. To prevent current flow from the drive wire to the drag wire, it is verified that tunneling between the two layers is negligible. The tunneling measurements are performed by sending a small source-drain voltage across the device for different top PO gate and bottom PO gate values, and then taking the numerical derivative of the resulting signal. Both top PO gate and bottom PO gate values were selected such that the tunneling resistance between the two wires was larger

than  $10M\Omega$  in a bias range of  $\pm 1.5\text{mV}$ . Two examples of tunneling measurement are shown in Fig. S3. Fig. S3(a) and Fig. S3(b) show the tunneling conductance across the two layers when the top PO gate is at  $-0.42\text{ V}$  and  $-0.44\text{ V}$ , respectively. The tunneling conductance is higher than  $10M\Omega$  when the top PO gate is at  $-0.44\text{ V}$  and the bottom PO gate is below  $-0.365\text{ V}$ .

The two scan windows are chosen to broaden the scanning subband configurations in crosstalking wires, as shown in Fig. S4. The wire conductance of the top and bottom wires in scan window 1 is shown in Fig. S4(d) and Fig. S4(e), respectively. The top wire has almost no crosstalk in scan window 1, and the bottom wire has relatively small crosstalk in the more conducting regions, which is confirmed by the slightly tilted vertical stripes in the detailed drag wire map, as shown in Fig. S5(a). For scan window 2, both wires have strong crosstalk, confirmed by the detailed scan of drag wire conductance, as shown in Fig. S5(b).

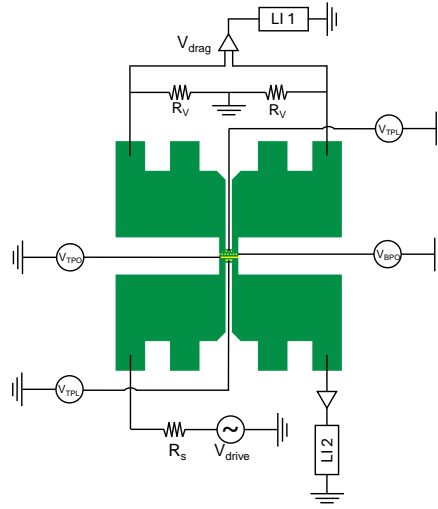

Fig. S2. **Measurement setup.** Circuit diagram for Coulomb drag measurements. A drive current is supplied to the top wire of the device and the drag voltage is measured in the bottom wire. The drive current is sourced using a  $R_s = 10M\Omega$  resistor in series with the drive wire. A virtual ground setup is used on the drag side of the experiment. Additionally, source-measure units are used to source and measure DC signals applied to the electrostatic gates.

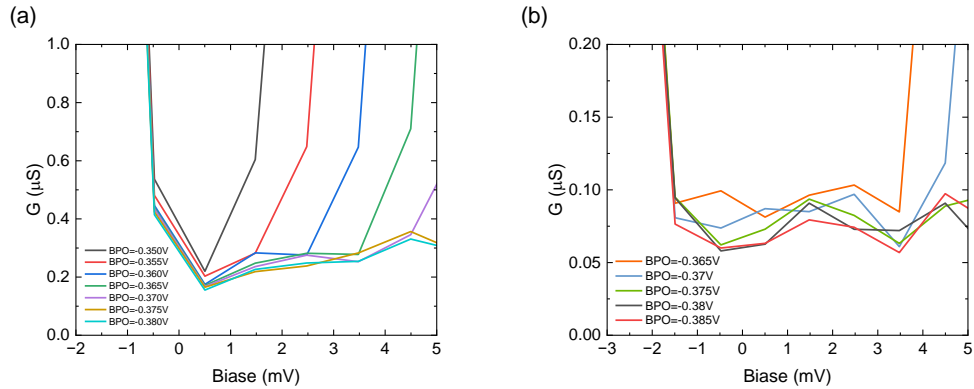

Fig. S3. **Example of a 2D-2D tunneling measurement.** The tunneling conductance is plotted against the source-drain bias across the tunnel barrier for various PO gate voltages. (a) The top PO gate at  $-0.42\text{V}$ , and (b) The top PO gate at  $-0.44\text{V}$ . The lines from top to bottom correspond to the bottom PO gate from  $-0.38\text{V}$  to  $-0.385\text{V}$ .

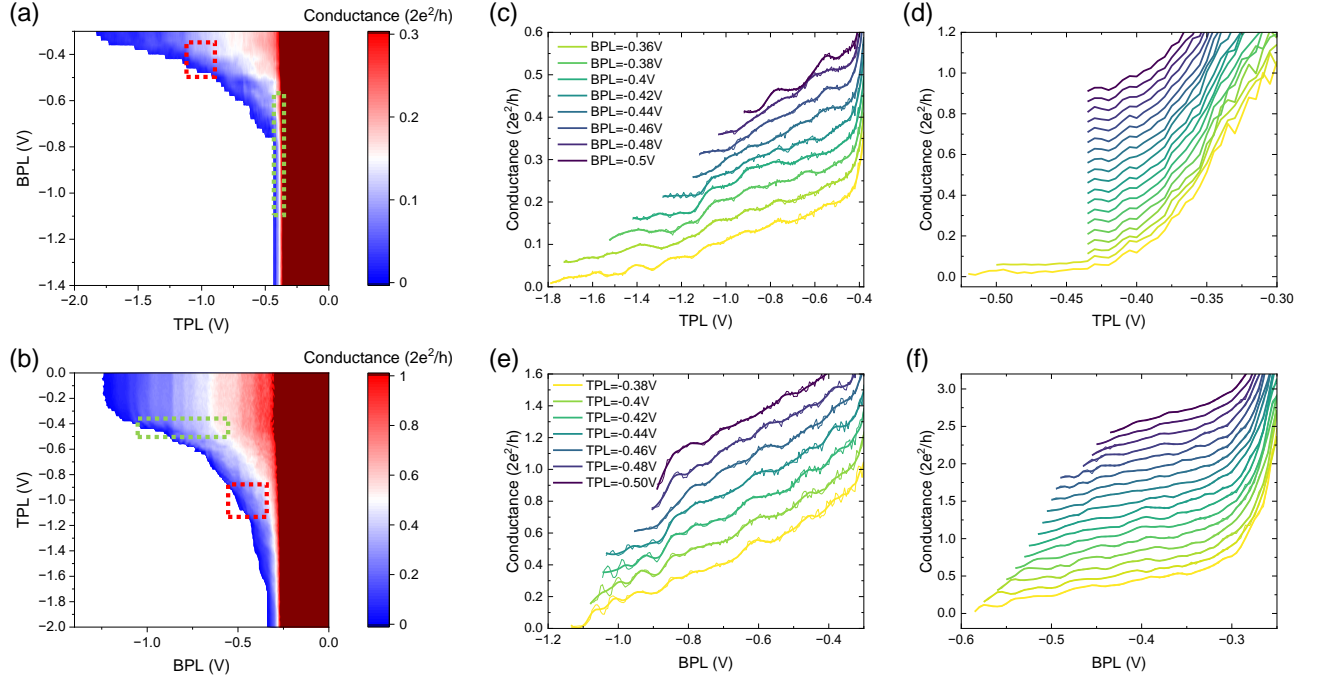

Fig. S4. **Wire conductance in scan windows 1 and 2.** (a, b) Wire conductance 2D maps for (a) the top (drive) wire, (b) the bottom (drag) wire. The green dotted box and red dotted box represent scan window 1 and scan window 2, respectively. (c, d) Wire conductance line cuts for the top wire at different BPL gate positions for (c) scan window 2, and (d) scan window 1. (e, f) Wire conductance line cuts for the bottom wire at different TPL gate positions for (e) scan window 1, and (f) scan window 2. Both wires have crosstalk in scan window 2 while the drive wire has almost no crosstalk in scan window 1.

### DRAG SIGNS AND CROSSOVER TEMPERATURES

Similar to Fig. 2, the correlation between the drag wire transconductance and the non-reciprocal drag signal is also verified in scan window 1, as shown in Fig. S5(c) and Fig. S5(d). The negative stripes of  $\frac{dG}{dV}$  of drag wire overlap with the positive  $V_{drag}^S$  corresponding to negative drag resistance, consistent with theory[2].

The 2D plot of  $V_{drag}^S$  and  $V_{drag}^{AS}$  as a function of the BPL gate voltage and the magnetic field for line cut TPL = -0.402 V is shown in Fig. S6. The two components have similar amplitude and sign changes as the drag wire subband changes. The spin splitting behavior is clear for both components.

The increase of crossover temperature in the spin-polarized regime can be confirmed with the gate-temperature 2D maps of  $\frac{dV_{drag}^{AS}}{dT}$  at 0 T and 14 T, as shown in Fig. S7. Similar to Fig. 4, the reciprocal drag signal shows a decrease in amplitude and an increase in the crossover temperature from 1.2 K at 0 T to  $\sim 1.7$  K at 14 T at line cut TPL = -0.402 V. Such a trend is also verified in line cut TPL = -1.095 V in scan window 2, as shown in Fig. S7(c) and Fig. S7(d).

### MAGNETIC FIELD DEPENDENT DRAG WIRE CONDUCTANCE

The magnetic field-dependent drag wire conductance 2D maps are shown in Fig. S8 and Fig. S9 for scan windows 1 and 2, respectively. In Fig. S8, the first subband stripe starts splitting around 2 T and completely splits around 8 T, while the initial two defect stripes have no splitting, confirming the physics origin of different stripes.

The B field dependent drag wire conductance is shown in Fig. S10 for TPL = -0.424 V. Similar to TPL = -0.402 V shown in Fig. 2(a), the initial two defect resonance peaks do not split with magnetic field increasing while the spin splitting of the first subband and the second subband start around 6 T, consistent with the subband assignment in Fig. 3.

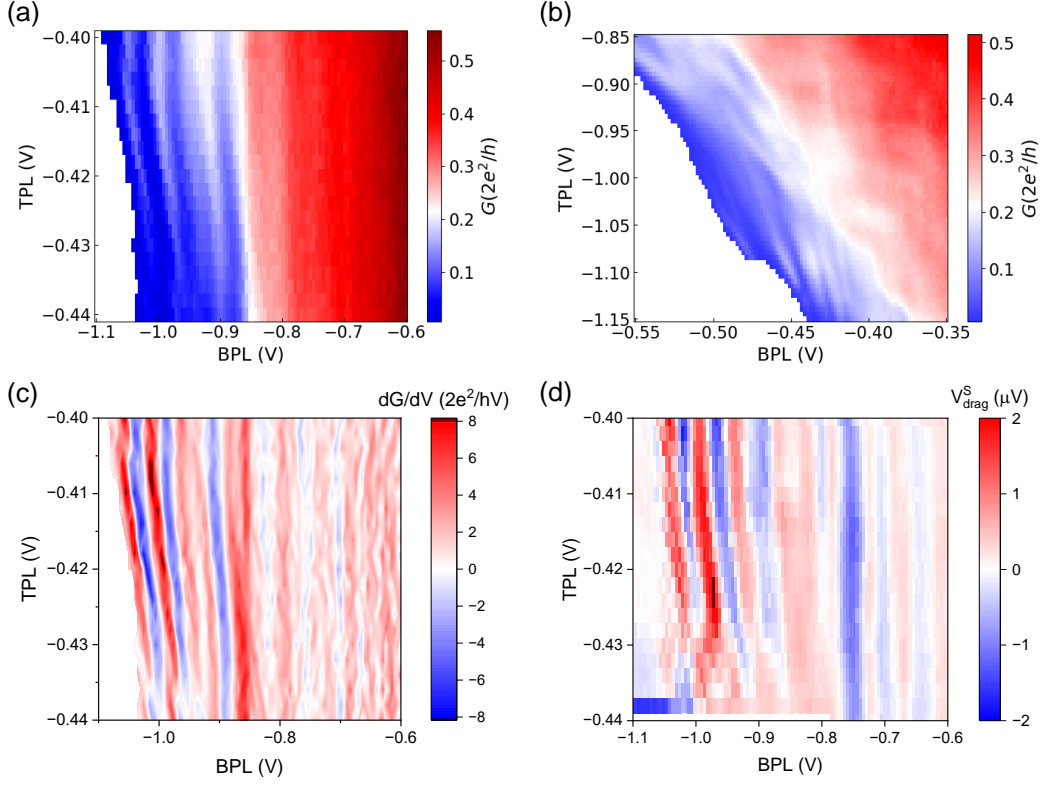

Fig. S5. **Wire conductance and drag sign.** (a, b) The wire conductance 2D maps as a function of the BPL and TPL gate positions of the bottom (drag) wire in (a) range 1 and (b) range 2. (c) The first derivative of the drag wire conductance over the BPL gate voltages as a function of the BPL and TPL gate positions. (d) The 2D plot of  $V_{drag}^S$  as a function of the BPL and TPL gate positions at base temperature. The negative stripes of  $\frac{dG}{dT}$  in (c) overlap with the positive stripes of  $V_{drag}^S$  in (d), consistent with Fig. 2.

### EXTRACTED $Kc-$ AT 0 T AND 14 T

The extracted  $Kc-$  at 0 T and 14 T for reciprocal and non-reciprocal components at three line cuts of scan window 1 and three line cuts in scan window 2 are shown in Fig. S11 and Fig. S12, respectively. The similar values of  $Kc-$ s at 0 T and 14 T are consistent with Fig. 3 and Fig. 4. The deviation and large error bars on the right of Fig. S11(a) and Fig. S11(d) are accounted for by the small signal amplitude in high subband regimes. The turning up of  $Kc-$  near the left tunneling regions is more obvious in  $TPL = -0.424$  V and  $TPL = -1.135$  V, where drag wire pinches off earlier than the other two line cuts, as shown in Fig. S5.

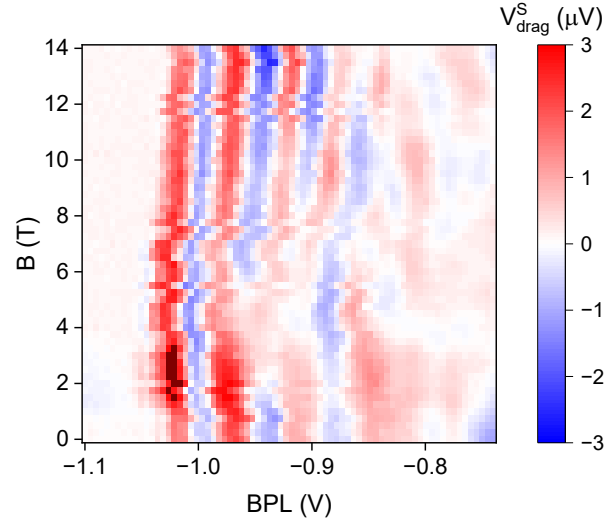

Fig. S6.  $V_{drag}^S$  **2D map at TPL = -0.402 V** The 2D plot of the symmetric component drag signal as a function of the BPL gate voltage and the magnetic field for line cut TPL = -0.402 V.

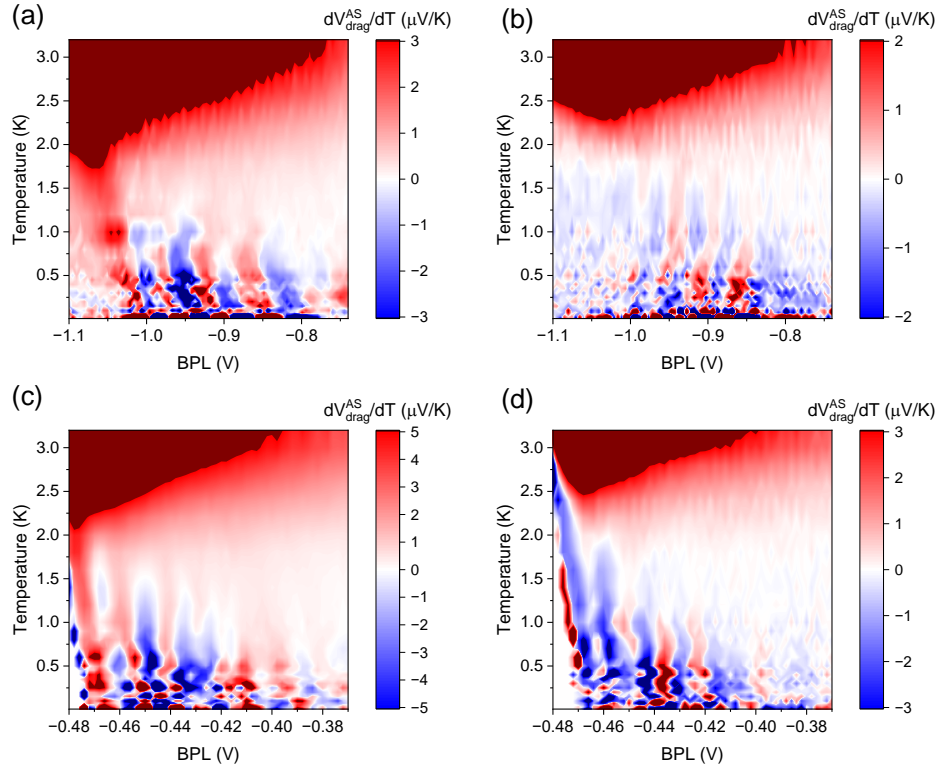

Fig. S7. **First derivative of  $V_{drag}^{AS}$**  (a, b) The first derivative of the antisymmetric component of Coulomb drag voltage  $V_{drag}^{AS}$  over temperature as a function of the BPL gate and temperature at (a) 0T and (b) 14T at line cut TPL = -0.402 V. The white regions around 1.2K in (a) and 1.75K in (b) represent the turning temperatures of the antisymmetric component of Coulomb drag. (c, d) The first derivative of the antisymmetric component of Coulomb drag voltage  $V_{drag}^{AS}$  over temperature as a function of the BPL gate and temperature at (a) 0T and (b) 14T at line cut TPL = -1.095 V.

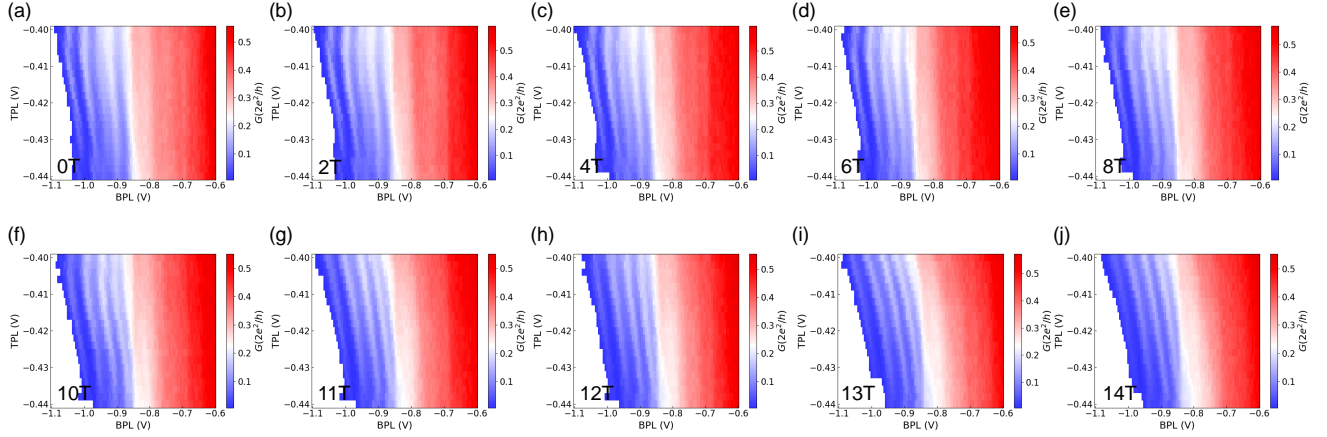

Fig. S8. **Magnetic field-dependent bottom wire conductance in the scan window 1.** (a-j) The bottom (drag) wire conductance 2D map in scan window 1 at the parallel magnetic field from 0 T to 14 T. The first subband spin splitting is clear with the stripe doubling.

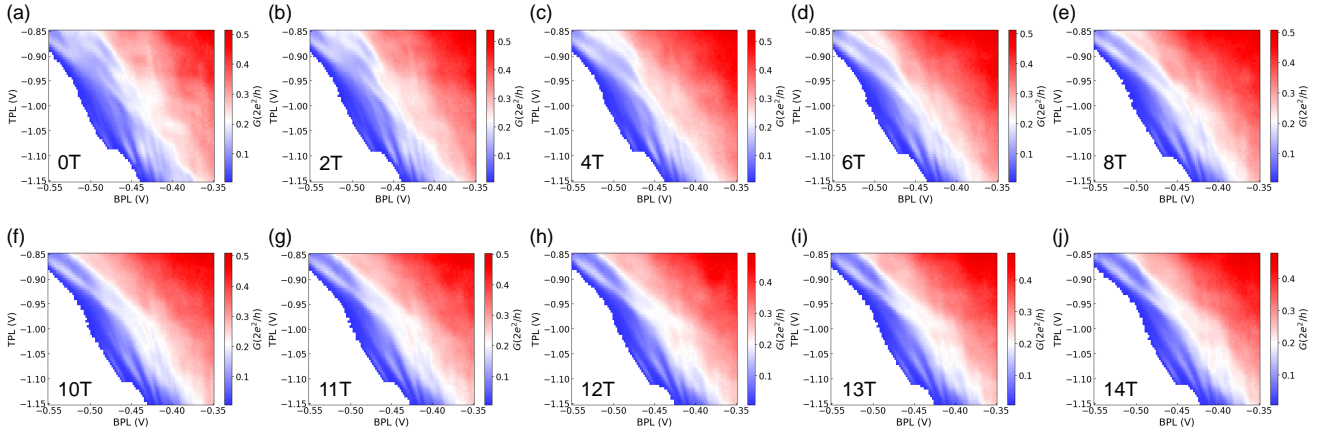

Fig. S9. **Magnetic field-dependent bottom wire conductance in the scan window 2.** (a-j) The bottom (drag) wire conductance 2D map in scan window 2 at the parallel magnetic field from 0 T to 14 T. The subband stripes are tilted because of the interwire crosstalk between the top and bottom wires.

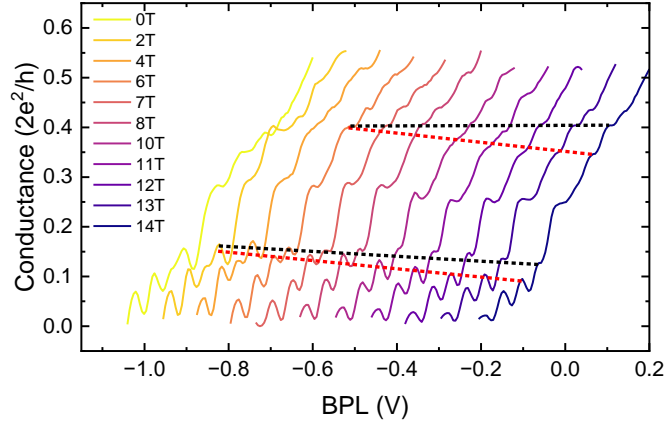

Fig. S10. **Spin polarization of wire conductance at TPL = -0.424 V.** Drag wire conductance as a function of the BPL gate voltage at the magnetic field from 0 T to 14 T when the TPL = -0.424 V. Successive lines are horizontally offset by 0.08 V for visibility. The 1D subband plateau features are seen clearly with the spin splitting as the magnetic field increases. The dotted lines are guides to the eye of the spin splittings of the first and second subbands.

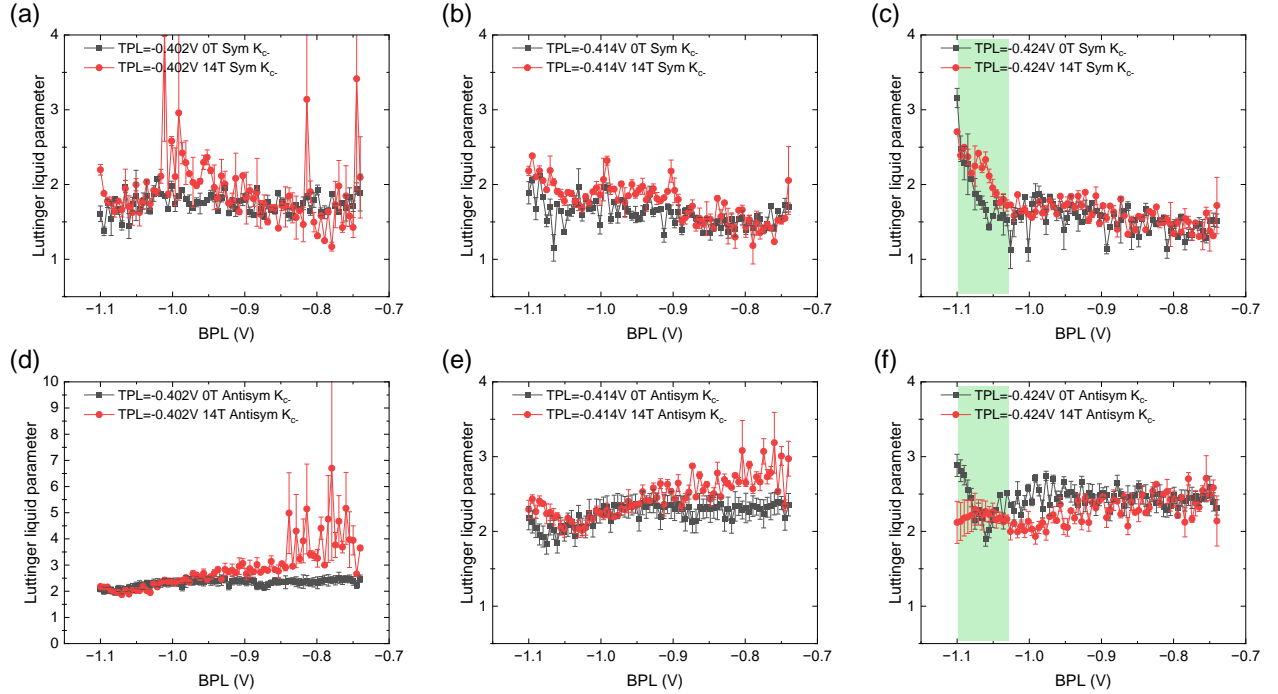

Fig. S11. **Extracted  $K_{c-}$  at 0 T and 14 T in scan window 1.** (a-c) The extracted  $K_{c-}$  for symmetric components at 0 T and 14 T for three line cuts at (a) TPL = -0.402 V, (b) TPL = -0.414 V, and (c) TPL = -0.424 V. (d-f) The extracted  $K_{c-}$  for antisymmetric components at 0 T and 14 T for three line cuts at (d) TPL = -0.402 V, (e) TPL = -0.414 V, and (f) TPL = -0.424 V. The shaded boxes represent the tunneling regions.

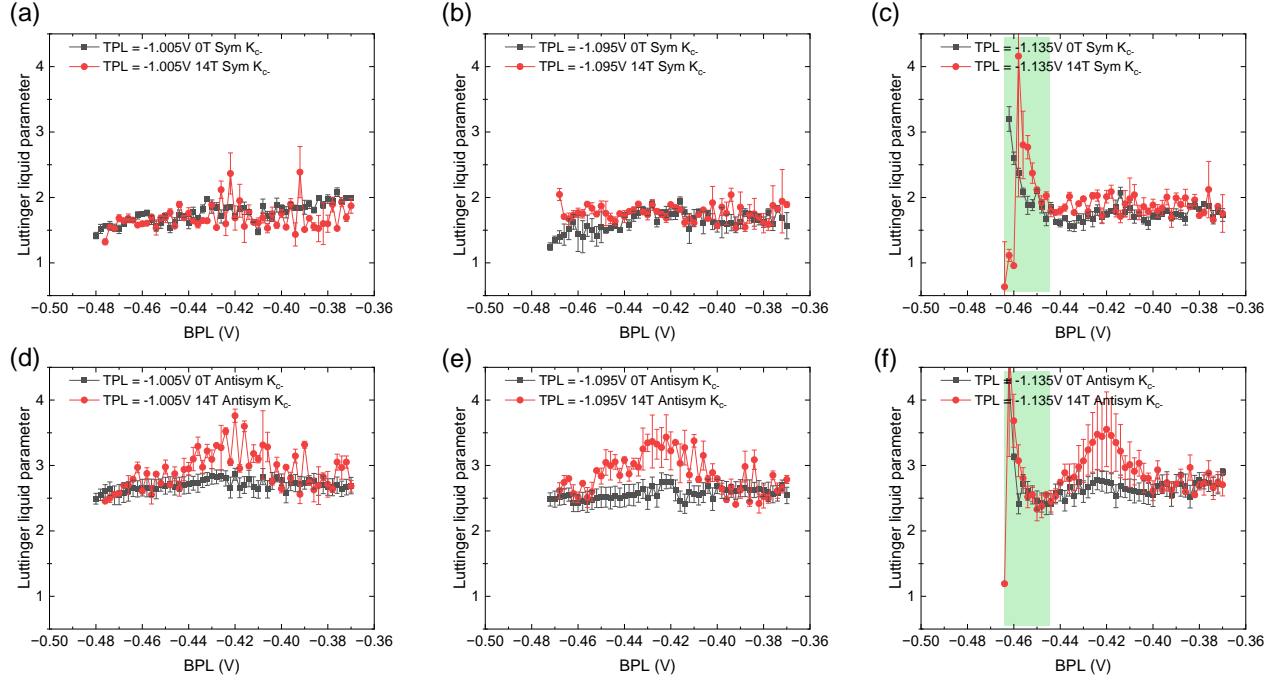

Fig. S12. **Extracted  $K_{c-}$  at 0 T and 14 T in scan window 2.** (a-c) The extracted  $K_{c-}$  for symmetric components at 0 T and 14 T for three line cuts at (a) TPL = -1.005 V, (b) TPL = -1.095 V, and (c) TPL = -1.135 V. (d-f) The extracted  $K_{c-}$  for antisymmetric components at 0 T and 14 T for three line cuts at (d) TPL = -1.005 V, (e) TPL = -1.095 V, and (f) TPL = -1.135 V. The shaded boxes represent the tunneling regions.

---

\* **Email of Author to whom correspondence should be addressed:** dlaroc10@ufl.edu

- [1] D. Laroche, G. Gervais, M. P. Lilly, and J. L. Reno, Positive and negative Coulomb drag in vertically integrated one-dimensional quantum wires, *Nature Nanotechnology* **6**, 793 (2011).
- [2] A. Levchenko and A. Kamenev, Coulomb drag in quantum circuits, *Physical Review Letters* **101**, 216806 (2008).
